# Supplementary material for: A single optically detectable tumbling spin in silicon
Source: arXiv:2510.15590 ancillary file (2026-01-29)
Supplement: Supplementary file 1 [file SI_single_tumbling_spin.pdf]

# A single optically detectable tumbling spin in silicon

## Supplementary Information

Félix Cache,<sup>1</sup> Yoann Baron,<sup>2</sup> Baptiste Lefaucher,<sup>3</sup> Jean-Baptiste Jager,<sup>3</sup>  
 Frédéric Mazen,<sup>2</sup> Frédéric Milési,<sup>2</sup> Sébastien Kerdilès,<sup>2</sup> Isabelle Robert-Philip,<sup>1</sup>  
 Jean-Michel Gérard,<sup>3</sup> Guillaume Cassabois,<sup>1,4</sup> Vincent Jacques,<sup>1</sup> and Anaïs Dréau<sup>1,\*</sup>  
<sup>1</sup>*Laboratoire Charles Coulomb, Université de Montpellier and CNRS, 34095 Montpellier, France*  
<sup>2</sup>*Université Grenoble Alpes, CEA-LETI, Grenoble 38000, France*  
<sup>3</sup>*Université Grenoble Alpes, CEA, Grenoble INP, IRIG, PHELIQS, 38000 Grenoble, France*  
<sup>4</sup>*Institut Universitaire de France, 75231 Paris, France.*

### I. G CENTER ACTIVATION WITH NANOFABRICATION AND DESTRUCTION WITH ANNEALING

Carbon and proton implantation fluences have been chosen to selectively create G centers with a density compatible with a mean number of defects per cavity around 1 (see Methods) [1]. Indeed, optical scans performed on the co-

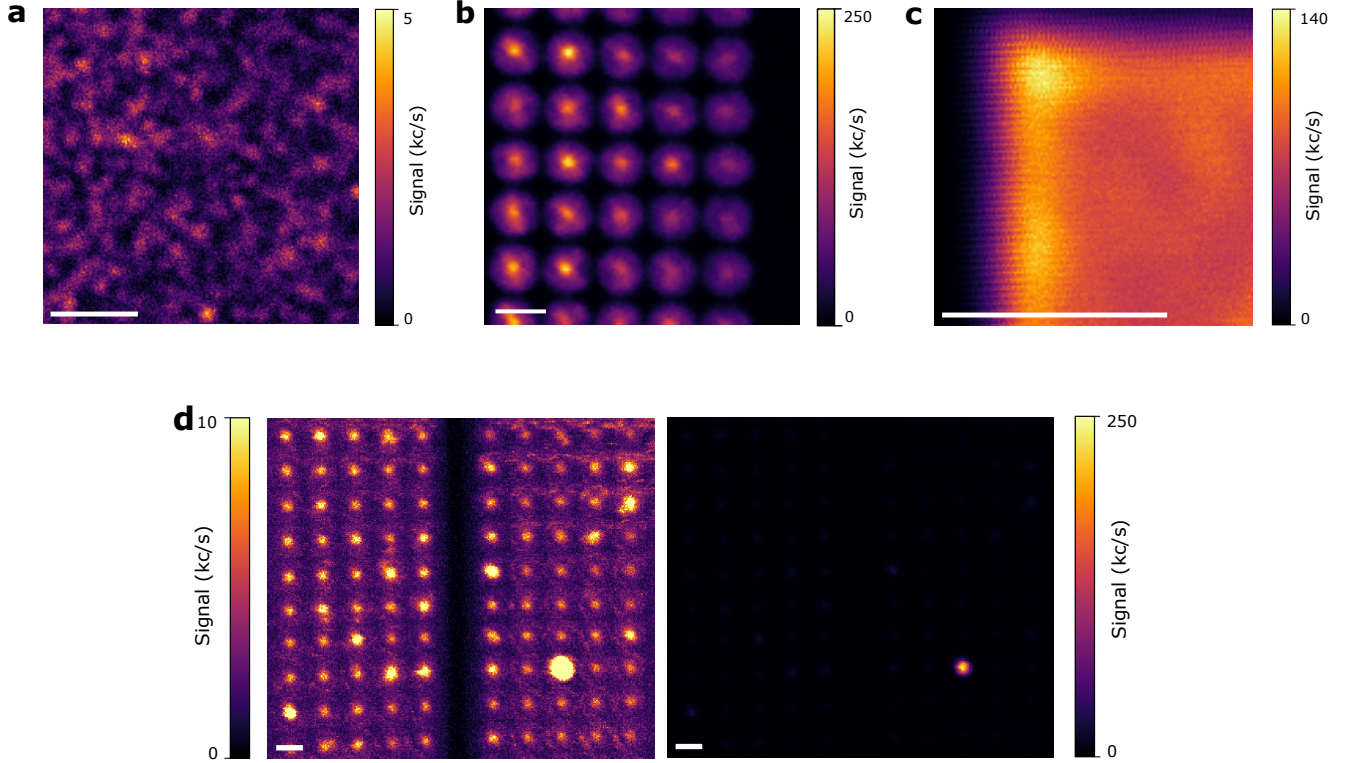

Figure. S1. **Impact of the fabrication steps on the G center density.** **a**, PL scans of the unpatterned SOI sample after the co-implantation process. Optical scans of the sample after nanofabrication around **b**, cavities with resonant mode at  $\sim 1274$  nm and **c**, a marker etched in the silicon layer recorded at 10  $\mu\text{W}$  and 60  $\mu\text{W}$ , respectively. **d**, PL image under 400  $\mu\text{W}$  of optical excitation of the SOI sample annealed at  $300^\circ\text{C}$  during 30 min after cavity fabrication, displayed with a color scale maximum set to 10 and 250  $\text{kc/s}$ , respectively. The cavity resonant mode is at  $\sim 1278\text{nm}$ , corresponding to the G center ZPL wavelength. The brightest hotspot corresponds to the single integrated G center from Figure 1 of the main text. White scale bars are 5  $\mu\text{m}$  for all scans.

\* [anaïs.dreau@umontpellier.fr](mailto:anaïs.dreau@umontpellier.fr)

implanted sample before nanostructuration show a spatially inhomogeneous PL signal, with an areal defect density of  $\sim 0.2 \mu\text{m}^{-2}$  (Fig. S1a). PL spectra confirm that all emitters are G centers. After nanofabrication, we observe that the core of all circular Bragg grating (CBG) cavities exhibit similar PL count rates, suggesting a high number of centers per cavity (Fig. S1b). To check the emitter density, we carry out optical scans on a nearby silicon marker of a few  $\mu\text{m}$  wide (Fig. S1c). Unlike the unstructured SOI sample (Fig. S1a), the PL signal is spatially homogeneous on the marker. Furthermore, the PL intensity, still associated to the G center emission, is particularly high, even though there is no enhancement of either the collection efficiency or the G radiative emission compared to unpatterned SOI. We can therefore conclude that nanofabrication has increased the G center density by several orders of magnitude. The G center activation by fabrication processes, already reported in literature for higher carbon concentration [2–4], is thus also valid for low carbon implantation fluence of  $1 \times 10^{10} \mu\text{m}^{-2}$ .

Since elevated temperatures are known to destroy G centers [5–8], we have annealed the SOI sample at  $300^\circ\text{C}$  during 30 min. PL image of the sample after annealing displays a drastic reduction of the emitter density, with strong fluctuations of photon counts between cavities (Fig. S1d). Spectral analysis indicates that only 43% of the CBG cavities still host G centers. Surprisingly, we found W center ZPL emission in 15% of the optical resonators [9, 10]. The G center areal concentration is estimated around  $\sim 0.02 \mu\text{m}^{-2}$ . This low density, combined with randomly located centers, leads to a very small probability to get a cavity with a well coupled G center [10]. Therefore, future works would require the deterministic control of the G defect position, for instance using implantation through masks with nanoholes [10, 11]. By restricting the carbon atoms to the center of the cavities, such method could prevent the unwanted activation of G centers during the nanofabrication step.

As rapid thermal annealing (RTA) at  $1000^\circ\text{C}$  during 20 s kills G centers [5, 6], this activation effect might have played a role in the G defect creation in the precedent demonstrations of photonic structures integrating single G centers that have all performed RTA before etching [11–16]. This has certainly contributed to the confusion between the  $G^*$  center that survives and is even activated by the RTA step, and the real G center in silicon that is destroyed with RTA, but can reform during the nanofabrication step [17].

## II. ADDITIONAL PL AND ODMR DATA

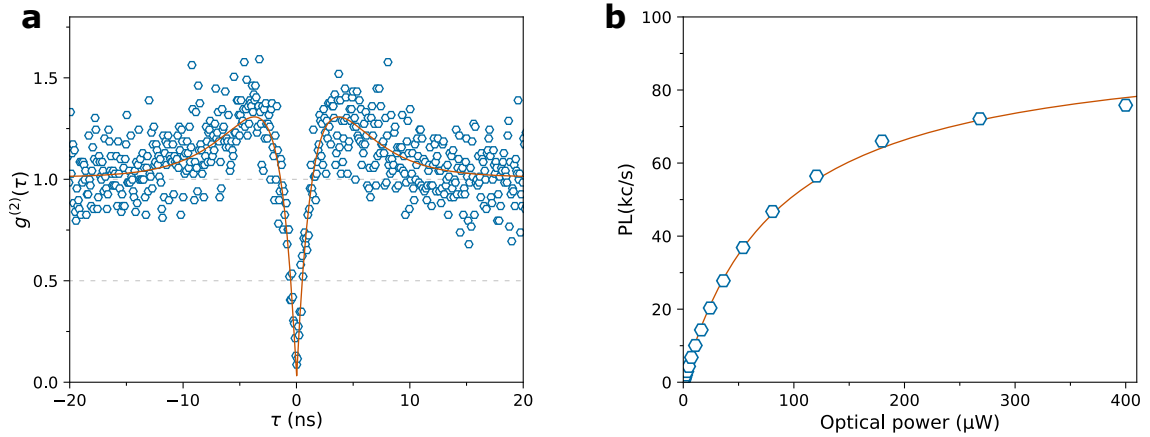

Figure. S2. **PL data on G#2.** **a**, Uncorrected autocorrelation function, providing  $g^{(2)}(0) = 0.10 \pm 0.05$ . Solid line is data fitting inferred from a rate equation model of a 3-level system [18]. **b**, Evolution of the PL counts with optical excitation power  $P$ . Dashed lines represent a fit to the data with standard saturation function:  $I_{\text{sat}}/(1 + P_{\text{sat}}/P)$ .

The G center G#1 whose optical data are presented in Figure 1 of the main text is the brightest integrated defect in our sample. However, it is located in the third cavity row away from the MW microstrip, which requires 9 times more microwave power for a given MW  $\pi$ -pulse compared to a G defect in a first-row cavity. To avoid heating issues, we therefore opted, for the spin data shown in the main text, for another G center G#2 integrated in a cavity closest to the MW stripline. This defect is also single, as evidenced by the antibunching at zero-delay observed in the uncorrected  $g^{(2)}$  function of Figure S2a:  $g^{(2)}(0) = 0.10 \pm 0.05$  (Fig. S2a). The maximum count rate recorded at saturation on G#2 is  $76 \text{ kcounts.s}^{-1}$  (Fig. 2b). As its cavity resonant mode is at  $\sim 1274 \text{ nm}$ , i.e. detuned by  $\sim 5 \text{ nm}$  from the G center ZPL wavelength, the PL enhancement observed on G#2 is mostly due to improved collection efficiency [10]. On the contrary, G#1, which is integrated in a CBG cavity resonant at  $\sim 1278 \text{ nm}$ , thus benefits from an increase of both the collection efficiency and its radiative rate by Purcell effect (Fig. 1d of main text).

Despite heating issues, we were able to measure the ODMR of G#1 associated to the spin transition  $|+\rangle \leftrightarrow |0\rangle$ . The ODMR spectrum of Figure S3, acquired with 110-ns long MW pulse, shows a fine spin structure with 3 lines. As the lower-frequency line features a contrast roughly twice higher than for the other two lines, it likely corresponds to two fine spin transitions close in energy (see Reorientation model in main text). Although the ODMR lines of this spectrum are power-broadened, we clearly observe that the transition frequencies and relative splittings of G#2 fine spin structure are different from the ones observed for G#1 (Fig. 3 of main text).

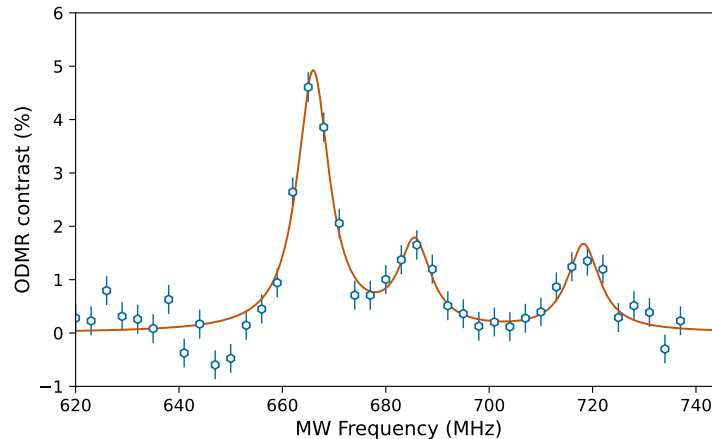

Figure. S3. **Fine spin structure on G#1.** ODMR spectrum recorded with a MW pulse duration of  $\sim 110$  ns on the spin transition  $|+\rangle \leftrightarrow |0\rangle$ .

- 
- [1] Y. Baron, A. Durand, T. Herzig, M. Khoury, S. Pezzagna, J. Meijer, I. Robert-Philip, M. Abbarchi, J.-M. Hartmann, S. Reboh, J.-M. Gérard, V. Jacques, G. Cassaboïs, and A. Dréau, *Applied Physics Letters* **121**, 084003 (2022).
  - [2] J. Weber, R. J. Davis, H. U. Habermeier, W. D. Sawyer, and M. Singh, *Applied Physics A Solids and Surfaces* **41**, 175 (1986).
  - [3] J. L. Benton, J. Michel, L. C. Kimerling, B. E. Weir, and R. A. Gottscho, *Journal of Electronic Materials* **20**, 643 (1991).
  - [4] S. G. Cloutier, P. A. Kossyrev, and J. Xu, *Nature Materials* **4**, 887 (2005).
  - [5] Y. Zhiyenbayev, W. Redjem, V. Ivanov, W. Qarony, C. Papapanos, J. Simoni, W. Liu, K. Jhuria, L. Z. Tan, T. Schenkel, and B. Kanté, *Optics Express* **31**, 8352 (2023).
  - [6] W. Redjem, Y. Zhiyenbayev, W. Qarony, V. Ivanov, C. Papapanos, W. Liu, K. Jhuria, Z. Y. Al Balushi, S. Dhuey, A. Schwartzberg, L. Z. Tan, T. Schenkel, and B. Kanté, *Nature Communications* **14**, 3321 (2023).
  - [7] A. M. Day, M. Sutula, J. R. Dietz, A. Raun, D. D. Sukachev, M. K. Bhaskar, and E. L. Hu, *Nature Communications* **15**, 4722 (2024).
  - [8] M. Hollenbach, N. Klingner, P. Mazarov, W. Pilz, A. Nadzeyka, F. Mayer, N. V. Abrosimov, L. Bischoff, G. Hlawacek, M. Helm, and G. V. Astakhov, *Advanced Quantum Technologies* **8**, 2400184 (2025).
  - [9] Y. Baron, A. Durand, P. Udvarhelyi, T. Herzig, M. Khoury, S. Pezzagna, J. Meijer, I. Robert-Philip, M. Abbarchi, J.-M. Hartmann, V. Mazzocchi, J.-M. Gérard, A. Gali, V. Jacques, G. Cassaboïs, and A. Dréau, *ACS Photonics* **9**, 2337 (2022).
  - [10] B. Lefaucher, Y. Baron, J.-B. Jager, V. Calvo, C. Elsässer, G. Coppola, F. Mazen, S. Kerdilès, F. Cache, A. Dréau, and J.-M. Gérard, *Bright single-photon source in a silicon chip by nanoscale positioning of a color center in a microcavity* (2025), arXiv:2501.12744 [physics].
  - [11] Y.-H. Ma, N.-J. Guo, W. Liu, X.-D. Zeng, L.-K. Xie, J.-Y. Liu, Y.-Q. Wu, Y.-T. Wang, Z.-A. Wang, J.-M. Ren, C. Ao, H. Lu, J.-S. Tang, C.-F. Li, and G.-C. Guo, *ACS Photonics* **12**, 5240 (2025).
  - [12] M. Prabhu, C. Errando-Herranz, L. De Santis, I. Christen, C. Chen, C. Gerlach, and D. Englund, *Nature Communications* **14**, 2380 (2023).
  - [13] V. Saggio, C. Errando-Herranz, S. Gyger, C. Panuski, M. Prabhu, L. De Santis, I. Christen, D. Ornelas-Huerta, H. Raniwala, C. Gerlach, M. Colangelo, and D. Englund, *Nature Communications* **15**, 5296 (2024).
  - [14] L. Komza, P. Samutpraphoot, M. Odeh, Y.-L. Tang, M. Mathew, J. Chang, H. Song, M.-K. Kim, Y. Xiong, G. Hautier, and A. Sipahigil, *Nature Communications* **15**, 6920 (2024).
  - [15] A. Buzzzi, C. Papon, M. Pirro, O. Hooybergs, H. Raniwala, V. Saggio, C. Errando-Herranz, and D. Englund, *Spectral tuning and nanoscale localization of single color centers in silicon via controllable strain* (2025), arXiv:2501.17290 [physics].
  - [16] K.-Y. Kim, C.-M. Lee, A. Boreiri, P. Purkayastha, F. Islam, S. Harper, J.-H. Kim, and E. Waks, *Nano Letters* **25**, 4347 (2025).

- [17] A. Durand, Y. Baron, F. Cache, T. Herzig, M. Khoury, S. Pezzagna, J. Meijer, J.-M. Hartmann, S. Reboh, M. Abbarchi, I. Robert-Philip, J.-M. Gérard, V. Jacques, G. Cassaboïs, and A. Dréau, [Physical Review B](#) **110**, L020102 (2024).
- [18] W. Redjem, A. Durand, T. Herzig, A. Benali, S. Pezzagna, J. Meijer, A. Y. Kuznetsov, H. S. Nguyen, S. Cuff, J.-M. Gérard, I. Robert-Philip, B. Gil, D. Caliste, P. Pochet, M. Abbarchi, V. Jacques, A. Dréau, and G. Cassaboïs, [Nature Electronics](#) **3**, 738 (2020).
